# Supplementary material for: Efficient Open World Reasoning for Planning
Source: arXiv:cs/0601032 source file (2006-09-26)
Supplement: Supplementary file 1 [file appendix-short.tex]

\section {Appendix}

\noindent {\bf Observation \ref{lm:unique}}
\restate{\lemmaOne}

{\begin{proof} %of Observation \ref{lm:unique}
The proof is by contradiction. Assuming there is a ground clause that is generated by more than one substitution on \m{\main(\psi)}, it is possible to construct a unifier for two literals of the main clause.
\ignore{ %long version of proof
Suppose \m{c} is a clause in \m{\psi}. If there are more than one
substitution on \m{\main(\psi)} that generate \m{c}, then it is the
case that two different literals of   \m{\main(\psi)} match onto the
same literal of \m{c}. Suppose  \m{\sigma_1} and
  \m{\sigma_2} are the substitutions corresponding to each set-match, and
that  they match two different
  literals \m{d_1} and \m{d_2} of \m{\main(\psi)} on the same
  literal \m{d} of \m{c}, i.e.  \m{d_1\sigma_1 = d_2\sigma_2 = d}.

Consider the following substitution \m{\sigma}.
\begin{itemize}
\item If \m{d_1} and \m{d_2} do not share variables, construct 
\m{\sigma} as follows: combine bindings on variables in \m{d_1} from
\m{\sigma_1} and  bindings on variables in \m{d_2} from \m{\sigma_2}.
Then, obviously, \m{d_1\sigma = d_2\sigma = d}.
  
\item Otherwise, if \m{d_1} and \m{d_2} do share variables, rename
variables in \m{d_2} so that there is no overlap with variables in
 \m{d_1}.  Modify \m{\sigma_2} by renaming the variables in the same
 way we did with  \m{d_2}, and construct \m{\sigma} as in the previous
 case. Again, \m{d_1\sigma = d_2\sigma}.
\end{itemize}

Thus, both cases produced a contradiction to the fact that no two
literals of a fixed length \m{\psi_1} unify.
}
\end{proof}
}

\ignore{
\noindent {\bf Observation \ref{lm:LitEntailment}}
\lemmaTwo

{\begin{proof} of Observation \ref{lm:LitEntailment}

Trivially follows from the definition of entailment.
% the proof below is omitted
\ignore{  (\m{\Rightarrow}) By contradiction. We have to show that
  \m{(c_1\entails c_2)\Rightarrow c_1\subseteq c_2}. Assume
  \m{(c_1\entails c_2)}, \m{c_1 = \set{d_1,\ldots,d_k}, c_2 =
    \set{d'_1,\ldots,d'_n}} and that \m{c_1\not\subseteq c_2}, i.e.
  \m{\ourexists{d_i}d_i\not\in c_2}.
  
  Consider the following interpretation \m{\cal I}.
  \ourmd{\begin{array}{l}
      {\cal I}(d_i) = \true \\
      {\cal I}(d_j) = \false, j\neq i, 1\leq j\leq k \\
      {\cal I}(d'_j) = \false, 1\leq j\leq n \\
       \end{array}
       } It is easy to see that \m{{\cal I}(c_1) = \true} and \m{{\cal
         I}(c_2) = \false}, which means that \m{c_1\not\entails c_2}.
     
     (\m{\Leftarrow}). We have to show that if \m{(c_1\subseteq c_2)}
     then \m{c_1\entails c_2}, i.e. every model of \m{c_1} is a model
     for \m{c_2}. This trivially follows from the fact that for any
     clause \m{c}, \m{\true \vee c} is equivalent to \m{ \true.}
}
\end{proof}
}
}
%%%% from psicalc file 

\noindent{\bf  Theorem \ref{th:clause-to-clause}.} 
\restate{\thrmOne}

\begin{proof} 
% of Theorem \ref{th:clause-to-clause}
(\m{\Rightarrow})A proof by contradiction is straightforward and thus omitted.
\ignore{
  We have to show that if \m{\Psi\entails\psi}, then
  \m{\ourforall{c\in\psi}\ourexists{c'\in\Psi}c'\entails c}.
  
  Suppose this is not true, i.e. there is a clause \m{c} in \m{\psi}
  which is not entailed by any clause in \m{\Psi}.
%% Let \m{c = \set{d_1, \ldots, d_n}}
  Consider the following interpretation \m{{\cal I}^0}: \m{{\cal I}^0}
  assigns \m{\true} to every literal of every clause of \m{\Psi}, and
  assigns \m{\false} to every other negated literal. Clearly, \m{{\cal
I}^0} is a model of \m{\Psi} and since \m{\Psi\entails\psi} it must 
  also be a model of \m{\psi}, i.e.  \m{{\cal I}^0(c) = \true}. Let
  \m{\set{d_{i_1},\ldots,d_{i_k}}} be the set of literals of \m{c} for
  which \m{{\cal I}^0(d_{i_j}) = \true, 1\leq j\leq k}. Clearly, this
  set is not empty, otherwise \m{{\cal I}^0(c)} would be \m{\false}.
  
  Now we construct an interpretation \m{{\cal I}^1} from \m{{\cal
      I}^0}.  \m{{\cal I}^1} is the same as \m{{\cal I}^0} except
  \m{{\cal I}^1(d_{i_1}) = \false}. If \m{{\cal I}^1(\Psi)} was equal
  to \m{\false} it would mean that there's a clause in \m{\Psi}, call
  it \m{c'}, that consists of just one literal, \m{d_{i_1}}, and
  therefore \m{c' \in c} and \m{c' \entails c}. So \m{{\cal
      I}^1(\Psi)} must be equal to \m{\true}.
  
  Let \m{{\cal I}^2} be the same as \m{{\cal I}^1} except \m{{\cal
      I}^1(d_{i_2}) = \false}. Again, if \m{{\cal I}^2(\Psi)} was
  equal to \m{\false} it would mean that there's a clause in \m{\Psi},
  call it \m{c'}, that consists of only two literals \m{d_{i_1}} and
  \m{d_{i_2}} and would thus be a subset of \m{c}. Thus, \m{{\cal
      I}^2(\Psi)} is \m{\true}.
  
  We continue this process until we build \m{{\cal I}^k}. Applying the
  same argument as for \m{{\cal I}^1} and \m{{\cal I}^2} to all
  \m{{\cal I}^j, 3\leq j\leq k} we conclude that \m{{\cal I}^k(\Psi) =
    \true}.  Clearly, \m{{\cal I}^k(c) = \false}, which means \m{\Psi}
  does not entail \m{c}, and therefore does not entail \m{\psi} We
  arrive at a contradiction.
}
  (\m{\Leftarrow}) Trivially follows from the definition of
  entailment.
\end{proof}

\noindent{\bf  Theorem \ref{th:SubsetMatch}} 
\restate{\thrmTwo}

{\begin{proof}% of Theorem \ref{th:SubsetMatch}

\noindent (\m{\Rightarrow})  \begin{sloppypar} 
Suppose
    \m{\psi_1\entails\psi_2}, \m{\main(\psi_1) = \set{\neg Q_1({\vec
          x_1}), \ldots, \neg Q_n({\vec x_n})}}, and \m{\main(\psi_2)
      = \set{\neg P_1({\vec y_1}), \ldots, \neg P_k({\vec y_k})}}.
    Assume \m{\mgusubset(\main(\psi_1), \main(\psi_2),
      \vars(\psi_1))=\emptyset}.
               \end{sloppypar}
                  
                  This means that for any substitution \m{\sigma} on
                  variables of \m{\psi_1}, there exists a literal in
                  \m{\main(\psi_1)\sigma}, which does not match any of
                  \m{\set{\neg P_1({\vec y_1}), \ldots, \neg P_k({\vec
                        y_k})}}. We can assume without any loss of
                  generality that the mismatched literal is \m{\neg
                    Q_1({\vec x_1})}.  Note that the mismatch can
                  occur due to one of the following reasons (we also
                  call them {\em mismatch types}):
\begin{enumerate}
\item \label{case1} the predicate denoted by \m{Q_1} is not the same
  as denoted by \m{P_i},
\item \label{case2} the argument list of \m{Q_1({\vec x_1})} has a
  constant, call it a {\em matching value}, at the position where
  \m{P_i({\vec y_i})}'s argument list has a variable, call it, a {\em
    mismatched variable}.
\item \label{case3} the argument list of \m{Q_1({\vec x_1})} has a
  constant, call it \m{B_i}, at the position where \m{P_i({\vec y_i})}
  has a different constant, \m{C_i}.
\end{enumerate} 
We now construct a clause from \m{\psi_2} and show that it cannot
contain as a subclause any clause of \m{\psi_1}. According to Theorem \ref{th:clause-to-clause} we would
then contradict the fact that \m{\psi_1 \entails \psi_2}.

Let \m{P'} be an instance of \m{\main(\psi_2)}, which is obtained by
assigning to each variable in \m{\vars(\psi_2)} a constant value which
does not occur anywhere in \m{\main(\psi_1)}. \edit{}{Since the number of constants in the language is infinite}, this can always be done. Since \m{\main(\psi_1)} does not
subset match onto \m{\main(\psi_2)}, it surely does not subset match
onto \m{P'}, because for any substitution \m{\sigma} on
\m{\vars(\psi_1)} the number of mismatches between any \m{Q} and any
literal of \m{P'} is at least the same as the number of mismatches
between a \m{Q} and a \m{P} in \m{\main(\psi_2)}, or higher, because
of the new mismatches of type \ref{case3}. Therefore, there is no
instance of \m{\main(\psi_1)} that is a subclause of \m{P'}.

(\m{\Leftarrow}) The existence of \m{\sigma} such that
\m{\main(\psi_1)\sigma\subseteq\main(\psi_2)} means that for every
ground clause \m{c_2} of \m{\psi_2}, assuming \m{c_2 =
  \main(\psi_2)\sigma'}, there is a clause \m{c_1} in \m{\psi_1},
\m{c_1 = \main(\psi_1)\sigma\sigma'}, which is a subset of \m{c_2},
and therefore \m{\psi_1\entails\psi_2}.
\end{proof}
}

\noindent{\bf  Theorem \ref{th:PreEntailmentthrm}}
\restate{\thrmThree}

{ \begin{proof}
 %of Theorem \ref{th:PreEntailmentthrm}

  We construct a clause of \m{\spsi{\main(\psi)}} and show that if
  none of \m{\spsi{\main(\psi_1)}, \ldots, \spsi{\main(\psi_n)}}
  entail it, then \m{\set{\psi_1, \ldots, \psi_n}} does not entail
  \m{\psi}.
  
  Suppose none of \m{\spsi{\main(\psi_1)}, \ldots,
    \spsi{\main(\psi_n)}} entail \m{\spsi{\main(\psi)}}.
  Therefore according to Theorem \ref{th:SubsetMatch} none of the main
  parts of these \psiforms{} subset match onto \m{\main(\psi)}.  Let
  \m{\sigma} be a substitution on \m{\vars(\psi)} that assigns to each
  variable a constant value that does not occur in any of \m{\psi_1,
    \ldots, \psi_n}, nor in the exceptions of \m{\psi}. This is always
  possible due to infinite number of constants in the language.  None of the
  clauses in \m{\main(\psi_1), \ldots, \main(\psi_n)} subset match
  onto \m{c=\main(\psi)\sigma}, because none of the main clauses of
  these \psiforms{} subsume \m{\main(\psi)} and the
  constants of \m{\sigma} do not appear in any of
  \m{\spsi{\main(\psi_1)}, \ldots, \spsi{\main(\psi_n)}}.  Thus,
  the clause \m{c=\main(\psi)\sigma} of \m{\psi} is not entailed by
  any clause in \m{\set{\spsi{\main(\psi_1)}, \ldots,
      \spsi{\main(\psi_n)}}}.  Since  \m{\Phi\subseteq
    \set{\spsi{\main(\psi_1)}, \ldots, \spsi{\main(\psi_n)}}},
  according to Theorem \ref{th:clause-to-clause} we conclude that
  \m{\Psi\not\entails \psi}. We arrive at a contradiction.
\end{proof}
}

\noindent{\bf  Theorem \ref{th:Entailmentthrm}.}
\restate{\thrmFour}

{ \begin{proof} 
% of Theorem  \ref{th:Entailmentthrm}
 
 The first requirement of this Theorem follows from Theorem
  \ref{th:PreEntailmentthrm}.  While the main part of \m{\psi_k} entails \m{\psi},
  the exceptions of \m{\psi_k} weaken \m{\psi_k}.  Thus, each clause
  in \m{\psi \diff \psi_k} must be entailed by some other \psiform{}
  in \m{\set{\psi_1,\ldots,\psi_{k-1},\psi_{k+1},\ldots,\psi_n}}.
\end{proof}
}

\noindent{\bf  Theorem \ref{th:SimpleImage-1}}
\thrmFive

{ \begin{proof} of Theorem \ref{th:SimpleImage-1}
It is easy to verify equality of the two sets by showing inclusion both ways.
\ignore{
  To show the equality of the two sets we show inclusion both ways. We
  denote the set of \psiforms{} on the right hand side of the equality
  by \m{\Psi}.
  
  \m{(\subseteq)} %We have to show that every ground clause in
  %\m{\psi_2} that is entailed by \m{\psi_1} is in \m{\Psi}.  
%Without  loss of generality, 
  Let \m{c_2} be a ground clause where \m{c_2 =
    \main(\psi_2)\sigma_2} such that \m{\psi_1\entails c_2}. According
  to Theorem \ref{th:SubsetMatch}, \m{\psi_1\entails c_2} means there
  exists a substitution \m{\sigma_1} on the variables of \m{\psi_1}
  such that \m{\main(\psi_1)\sigma_1 \subseteq c_2}.  Let \m{\sigma =
    \sigma_1\sigma_2}. Since each of \m{\sigma_1, \sigma_2} only bind
  the variables of \m{\psi_1} and \m{\psi_2} respectively, we have
  \m{c_2 = \main(\psi_2)\sigma} and consequently \m{\main(\psi_1)\sigma \subseteq  \main(\psi_2)\sigma}, i.e. \m{\sigma} is an instance of some most general subset unifier in \m{
      \mgusubset(\main(\psi_1),\main(\psi_2))}. This implies that
  \m{c_2 \in \Psi}.
  
  \m{(\supseteq)} We have to show that every clause in \m{\Psi} is in
  \m{\psi_2} and is entailed by \m{\psi_1}. The first part is obvious.
  The second follows from the definition of the \m{\mgusubset}: for
  each \m{\sigma \in{\mgusubset(\main(\psi_1),\main(\psi_2))}},
  \m{\main(\psi_1)\sigma \subseteq \main(\psi_2)\sigma}, i.e. every
  ground clause \m{c_2= \main(\psi_2)\sigma\sigma_2} contains as a
  subclause the clause of \m{\psi_1}, namely
  \m{\main(\psi_1)\sigma\sigma_2}.
}
  \end{proof}
}

\noindent{\bf  Theorem \ref{th:SimpleDiff}}
\restate{\thrmSix}

{\begin{proof} % of Theorem \ref{th:SimpleDiff}

  To prove this theorem we use Theorem \ref{th:SimpleImage-1} and the
  equality \m{\psi_2 \diff \psi_1 = \psi_2 - ({\image
      {\psi_1}{\psi_2}})}.
  
\noindent According to definition (\ref{def:psiformset-b})
% and (\ref{def:setoperations}) \marnote{check these refs}
 \md{[\main(\psi_2)\mbox{ except }\subst(\psi_2)\cup\Sigma'] =
	%% {\spsi{\main(\psi_2)\ourst\subst(\psi_2)\wedge\Sigma'}} =
    \spsi{\main(\psi_2)} - \exc(\psi_2) -
    \spsi{\main(\psi_2)\sigma_1'} - \ldots -
    \spsi{\main(\psi_2)\sigma_n'}, } where \m{\Sigma' =
    \set{\sigma_1',\ldots,\sigma_n'}}. Note that
  \m{\spsi{\main(\psi_2)} - \exc(\psi_2) = \psi_2}, and that
  \m{\spsi{\main(\psi_2)\sigma'_1}\cup\ldots\cup
    \spsi{\main(\psi_2)\sigma'_n}= {\image
      {\psi_1}{\spsi{\main(\psi_2)}}}}, and thus \md{
    [\main(\psi_2)\mbox{ except }\subst(\psi_2)\cup\Sigma'] = \psi_2 -
    ({\image {\psi_1}{\spsi{\main(\psi_2)}}}). }  It remains to
  show that
\begin{equation}\label{eq:loc}
\psi_2 -  ({\image {\psi_1}{\spsi{\main(\psi_2)}}}) = 
\psi_2 -  ({\image {\psi_1}{\psi_2}}).
\end{equation}
%and from that we'll be able to conclude \md{
%[\main(\psi_2)\mbox{ except }\subst(\psi_2)\cup\Sigma'] = \psi_2 -
%  ({\image {\psi_1}{\psi_2}}) = \psi_2 \diff \psi_1.  }
 Indeed
\m{({\image {\psi_1}{\psi_2}}) = ({\image
    {\psi_1}{\spsi{\main(\psi_2)}}}) - ({\image
    {\psi_1}{\exc(\psi_2)}}).}  Substituting the right hand side
instead of \m{({\image {\psi_1}{\psi_2}})} in (\ref{eq:loc}), we get
\md{ \psi_2 - ({\image {\psi_1}{\spsi{\main(\psi_2)}}}) = \psi_2 -
 [ ({\image {\psi_1}{\spsi{\main(\psi_2)}}}) - ({\image
    {\psi_1}\exc(\psi_2)}) ] } Since \m{({\image
    {\psi_1}{\exc(\psi_2)}})} is in \m{\exc(\psi_2)} and therefore
definitely not in \m{\psi_2}, \md{
\psi_2 - ({\image {\psi_1}{\spsi{\main(\psi_2)}}}) =
  \psi_2 - [({\image
    {\psi_1}{\spsi{\main(\psi_2)}}}) - ({\image
    {\psi_1}{\exc(\psi_2)}})] = \psi_2 - ({\image
    {\psi_1}{\spsi{\main(\psi_2)}}}) } We have arrived at a
tautology, which proves (\ref{eq:loc}).  
\end{proof}
}

\noindent {\bf Lemma \ref{lm:Image}}
\lemmaThree

{\begin{proof} %of Lemma \ref{lm:Image}

  Let \m{A={\image {\spsi{\main(\psi_1)}}
      {\spsi{\main(\psi_2)}}}}.  We substitute the definition of \m{
    H(\psi_1,\psi_2)} from (\ref{def:holes}) on the right hand side.
  
  \md{{\image{\psi_1}{\psi_2}} =  A-(A-({\image{\psi_1}{\spsi{\main(\psi_2)}} }))-
    \exc(\psi_2)}
  
  When \m{X,Y} and Z denote arbitrary sets, we have
\begin{equation}\label{eq:sets1}
X-(Y-Z) = (X-Y)\cup(X\cap Y\cap Z),
\end{equation} so
%\md{
%\begin{array}{c}
%{\image{\psi_1}{\psi_2}} = 
%{(A-A)\cup(A\cap A \cap ({\image{\psi_1}{\spsi{\main(\psi_2)}} }))} -
%\exc(\psi_2) = \\
%(A\cap ({\image{\psi_1}{\spsi{\main(\psi_2)}} })) - \exc(\psi_2) = \\
%({\image{\psi_1}{\spsi{\main(\psi_2)}} }) - \exc(\psi_2) =  \\
% {\image{\psi_1}{(\spsi{\main(\psi_2)} - \exc(\psi_2) )} } =
% {\image{\psi_1}{\psi_2}} 
%   \end{array}
%   } 
\md{\eqalign{
     \image{\psi_1}{\psi_2} 
={}& {(A-A)\cup(A\cap A \cap ({\image{\psi_1}{\spsi{\main(\psi_2)}} }))} -
     \exc(\psi_2) \cr
={}& (A\cap ({\image{\psi_1}{\spsi{\main(\psi_2)}} })) - \exc(\psi_2)
     \cr
={}& ({\image{\psi_1}{\spsi{\main(\psi_2)}} }) - \exc(\psi_2) \cr
={}&  {\image{\psi_1}{(\spsi{\main(\psi_2)} - \exc(\psi_2) )} } \cr
={}&  {\image{\psi_1}{\psi_2}} 
}} 
\end{proof}
}

\noindent {\bf Lemma \ref{lm:Diff}}
\lemmaFour

{\begin{proof}% of Lemma \ref{lm:Diff}

  From Lemma \ref{lm:Image} and equivalence (\ref{eq:DiffImg}) we have
  \m{\psi_2\diff\psi_1 = \psi_2-(\image{\psi_1}{\psi_2})}, or
  \md{\begin{array}{c}

\psi_2 \diff \psi_1 = 
\underbrace{\psi_2}_A - 
[(\underbrace{({\image {\spsi{\main(\psi_1)}} {\spsi{\main(\psi_2)}}})}_B - \underbrace{H(\psi_1,\psi_2)}_C) - \underbrace{\exc(\psi_2)}_D] 
    \end{array}
    } \ignore{ Since for any sets \m{A,B} and \m{C}, \m{A-(B-C) =
      (A-B)\cup(A\cap B \cap C)} we have \md{\begin{array}{c}
        A-((B-C)-D) = (A-(B-C))\cup(A\cap (B-C) \cap D)
   \end{array}
   }}

Using (\ref{eq:sets1}), we rewrite the right hand side equivalently \md{
  \psi_2\diff\psi_1= A-((B-C)-D) = (A-(B-C))\cup(A\cap (B-C) \cap D) }

Since in our case \m{A\cap D =\emptyset}, therefore \m{(A\cap (B-C)
  \cap D)= \emptyset} and we get \md{ \psi_2 \diff \psi_1 = (A-(B-C))
  = (A-B)\cup(A\cap B \cap C)}

We now evaluate \m{A\cap B\cap C}.  We note that \m{A\cap B=
  ([\main(\psi_2)] - D)\cap B } and since \m{(X-Y)\cap Z = X\cap Z -
  Y\cap Z}, we have \md{A\cap B= [\main(\psi_2)]\cap B - D\cap B =
  B-B\cap D = B-D.}

Next, \m{(B-D)\cap C = B\cap C -D\cap C} and since \m{C\subseteq B},
\m{(B-D)\cap C = C -D\cap C = C-D,} so we get

%\mbox {( since \m{(A\cap B = (B-D))} and \m{(B-D)\cap C =(C-D)}, because
%\m{C\subseteq B})}

%\md{\begin{array}{c}
%    \psi_2\diff\psi_1=(A-B)\cup(C-D) = \\
%    (\psi_2 - ({\image {\spsi{\main(\psi_1)}}
%      {\spsi{\main(\psi_2)}}})) \cup ( H(\psi_1,\psi_2) - \exc(\psi_2)) = \\
%    (\spsi{\main(\psi_2)} - \exc(\psi_2) - ({\image
%      {\spsi{\main(\psi_1)}}
%      {\spsi{\main(\psi_2)}}})) \cup ( H(\psi_1,\psi_2) - \exc(\psi_2)) = \\
%    ({\spsi{\main(\psi_2)}} \diff {\spsi{\main(\psi_1)}} -
%    \exc(\psi_2))
%    \cup ( H(\psi_1,\psi_2) - \exc(\psi_2))=\\
%    (({\spsi{\main(\psi_2)}} \diff {\spsi{\main(\psi_1)}}) \cup
%    H(\psi_1,\psi_2)) - \exc(\psi_2).
%    \end{array}
%    }
\md{\eqalign{
     \psi_2\diff\psi_1
={}& (A-B)\cup(C-D) \cr
={}& (\psi_2 - ({\image {\spsi{\main(\psi_1)}}
      {\spsi{\main(\psi_2)}}})) \cup ( H(\psi_1,\psi_2) -
     \exc(\psi_2)) \cr
={}& (\spsi{\main(\psi_2)} - \exc(\psi_2) - ({\image
      {\spsi{\main(\psi_1)}}
      {\spsi{\main(\psi_2)}}})) \cup ( H(\psi_1,\psi_2) -
     \exc(\psi_2)) \cr
={}& ({\spsi{\main(\psi_2)}} \diff {\spsi{\main(\psi_1)}} - \exc(\psi_2))
    \cup ( H(\psi_1,\psi_2) - \exc(\psi_2)) \cr
={}& (({\spsi{\main(\psi_2)}} \diff {\spsi{\main(\psi_1)}}) \cup
    H(\psi_1,\psi_2)) - \exc(\psi_2).
}}
\end{proof}
}

\noindent{\bf  Theorem \ref{th:emptyImage}}
\thrmSeven

{\begin{proof} %of Theorem \ref{th:emptyImage}

  As follows from Theorem \ref{th:SimpleImage-1},   
\m{\mgusubset(\main(\psi_1), \main(\psi_2)) = \emptyset} implies that
the image  \m{\image {\spsi{\main(\psi_1)}} {\spsi{\main(\psi_2)}}}
is empty. Since \m{(\image{\psi_1}{\psi_2} )\subseteq ({\image
{\spsi{\main(\psi_1)}} {\spsi{\main(\psi_2)}}})}, we have that 
\m{\image{\psi_1}{\psi_2} = \emptyset}  and therefore  
by equivalence (\ref{eq:DiffImg}) \m{\psi_2 \diff \psi_1 =  \psi_2}.
\end{proof}
}

\noindent{\bf  Theorem \ref{th:all1}}
\thrmEight
{\begin{proof} %of Theorem \ref{th:all1}

  (\ref{th:case2Img}) and (\ref{th:case2Diff}) trivially follow from
  Lemma \ref{lm:Image} and definition (\ref{def:holes}) by substituting
  \m{\spsi{\main(\psi_2)}} in place of
  \m{\image{\spsi{\main(\psi_1)}}{\spsi{\main(\psi_2)}}} and
  substituting \m{\emptyset} in place of
  \m{{\spsi{\main(\psi_1)}}\diff{\spsi{\main(\psi_2)}}}. 

\end{proof}
}

%\begin{ourlemma}\label{lm:aux}
%\lemmaFive
%\end{ourlemma}
\noindent {\bf Lemma \ref{lm:aux}}\lemmaFive 

{\begin{proof} % of Lemma \ref{lm:aux}
 Each \m{\psi_1^i} entails
  \m{\spsi{\main(\psi_2)}}, i.e.  \m{\image {\psi_1^i}{
      \spsi{\main(\psi_2)}} = {\spsi{\main(\psi_2)}}} for each \m{1\leq
    i\leq{\norm{\Theta}}}, because the main clause of each \m{\psi_1^i}
%  matches onto 
equals some subset of literals of \m{\main(\psi_2)}. However,
 each \m{\psi_1^i} may contain clauses that are exceptions of
  \m{\psi_1}, namely \m{\bigcup_{j=0}^{\norm\Sigma(\psi_1)}
  {(\spsi{\exci{j}(\psi_1)}\cap \psi_1^i)}}. We call these clauses 
{\em \m{\psi_1}'s exceptions in  \m{\psi_1^i} }.

  Thus, \m{\setpsi(\Psi_1)} contains all clauses of \m{\psi_1} that entail
  something in \m{\spsi{\main(\psi_2)}} and more, namely
  \m{\psi_1}'s exceptions in  \m{\psi_1^i}.  Therefore  
  \md{{\image {\psi_1}{\spsi{\main(\psi_2)}}} =   
  \bigcup_{\psi_1^i\in\Psi_1}({\image {({\psi_1^i} - \cup_{j=0}^{\norm{\Sigma(\psi_1)}}(\spsi{\exci{j}(\psi_1)}\cap
  \psi_1^i))} {\spsi{\main(\psi_2)}}}).}  
 Note that for a given \m{\psi_1^i\in\Psi_1}, each clause of
  \m{{ \spsi{\main(\psi_2)}}} is entailed by exactly
  one clause of \m{\psi_1^i}, i.e. for every \m{\psi_1^i\in\Psi_1}, and
  every \m{c\in  \spsi{\main(\psi_2)}, (\psi_1^i
    \entails c) \Leftrightarrow \ourexists{!c_1 \in \psi_1^i}
    {c_1\entails c}}
  (existence of a clause 
   \m{ \main(\psi_2)\sigma} such that there are 2 different clauses
  \m{c',c''\in\psi_1^i} that entail it, leads to a contradiction to the
  fact that \m{\psi_2} and \m{\psi_1} are fixed length \psiforms).
 The last observation allows to distribute the image operator and rewrite the last   expression as follows
%\md{
%\begin{array}{c}
%{\image {\psi_1}{\spsi{\main(\psi_2)}}} =   
%  \bigcup_{\psi_1^i\in\Psi_1}(({\image {\psi_1^i}{\spsi{\main(\psi_2)}}}) -
% {\image {\bigcup_{j=0}^{\norm{\Sigma(\psi_1)}}(\spsi{\exci{j}(\psi_1)}\cap
%  \psi_1^i)} {\spsi{\main(\psi_2)}} }) \\=
%  {\spsi{\main(\psi_2)}}  - \bigcap_{\psi_1^i\in\Psi_1}\bigcup_{j=0}^{\norm{\Sigma(\psi_1)}} ({\image
%{(\spsi{\exci{j}(\psi_1)}\cap \psi_1^i )}
%{\spsi{\main(\psi_2)}}}).
%\end{array}
\md{\eqalign{
     \image {\psi_1}{\spsi{\main(\psi_2)}}
={}& \bigcup_{\psi_1^i\in\Psi_1}\Bigl(({\image {\psi_1^i}{\spsi{\main(\psi_2)}}}) -
 {\image {\bigcup_{j=0}^{\norm{\Sigma(\psi_1)}}(\spsi{\exci{j}(\psi_1)}\cap
  \psi_1^i)} {\spsi{\main(\psi_2)}} }\Bigr) \cr
={}& {\spsi{\main(\psi_2)}}  - \bigcap_{\psi_1^i\in\Psi_1}\bigcup_{j=0}^{\norm{\Sigma(\psi_1)}} \bigl({\image
{(\spsi{\exci{j}(\psi_1)}\cap \psi_1^i )}
{\spsi{\main(\psi_2)}}}\bigr).
}
} i.e. the set of clauses of \m{\spsi{\main(\psi_2)}} not entailed by
 \m{\psi_1}  is  the {\em intersection} of images
 of \m{\psi_1}'s exceptions  in {\em all} of \m{\psi_1^i\in\Psi_1},

The formula for \m{H(\psi_1, \psi_2)} follows from substituting the
derived expression for \m{\image {\psi_1}{\spsi{\main(\psi_2)}}} in
the definition (\ref{def:holes}) and noticing that since \m{\psi_1}
nearly entails \m{\psi_2},
\m{\image{\spsi{\main(\psi_1)}}{\spsi{\main(\psi_2)}} =
{\spsi{\main(\psi_2)}}}. 
\end{proof}
}

\noindent {\bf Observation \ref{lm:varnum}}\lemmaSix

\begin{proof} % of Observation \ref{lm:varnum}

%Follows from the  results of Theorems \ref{th:SimpleImage-1},\ref{th:all1}  and Lemma \ref{lm:aux}).

As follows from  Theorem \ref{th:all1}  and  Lemma \ref{lm:aux} the e-difference is a subset of a union of images of exceptions of \m{\psi_1} on \m{\spsi{\main(\psi_2)}}. Each such image 
is obtained by instantiating the main clause \m{\main(\psi_2)} with a subset unifying substitution, call it \m{\sigma}. When \m{\sigma} does not bind any variables of \m{\psi_2} to constants, the image is equal to \m{\spsi{\main(\psi_2)}}, which contradicts the conditions of the Observation.   Thus, \m{\sigma} must bind some variables of \m{\main(\psi_2)} to constants, and therefore 
\m{\spsi{\main(\psi_2)\sigma}}, and in turn, every subset of this \psiform{} is  expressed with a \psiform{} that contains strictly fewer variables than \m{\spsi{\main(\psi_2)}}  
 \end{proof}

\noindent{\bf  Theorem \ref{th:FLImageDiff}}
\thrmNine
{\begin{proof}% of Theorem \ref{th:FLImageDiff}

By Theorem \ref{th:SimpleImage-1} \m{\mgusubset(\main(\psi_1),\main(\psi_2))\neq\emptyset} implies that 
the image \m{\Psi} %= {\image{\spsi{\main(\psi_1)}}{\spsi{\main(\psi_2)}}}} 
is non-empty and thus consists of a set of simple \psiforms{}. Each 
\psiform{} in \m{\Psi} is nearly entailed by \m{\psi_1}. 
The image \m{\image {\psi_1} {\psi_2}} is a subset of \m{\Psi}, and
equals exactly the set of all clauses in \m{\Psi} that are not exceptions of
\m{\psi_2} and that are entailed by \m{\psi_1}, i.e.
\md{{\image {\psi_1} {\psi_2} = ({\image {\psi_1} {\Psi}}) - \exc(\psi_2)
}.} Since each of \psiforms{} in \m{\Psi} is nearly entailed by
\m{\psi_1} the calculation of the image \m{\image {\psi_1} {\Psi}}  in the above expression can be
carried out according to Theorem \ref{th:all1}.

The proof of (\ref{th:FLDiff}) is similar. The part of \m{\psi_2} that
is not entailed by \m{\psi_1} includes \m{\psi_2 - \Psi} plus parts of 
\m{\Psi} that are not exceptions of \m{\psi_2} and are not entailed by \m{\psi_1}, i.e. \m{(\Psi  - \exc(\psi_2)) \diff {\psi_1}}. 
\end{proof}
}

\noindent{\bf  Theorem \ref{th:thelast}}
\thrmTen

{\begin{proof} %of Theorem \ref{th:thelast}

  The fact that all operations produce sets of \psiforms{} follows
  from the fact that all of them produce subsets of operand \psiforms.
  The fact that indeed this set is finite follows from the Theorems
  \ref{th:emptyImage}, \ref{th:FLImageDiff}.
  
  The resulting \psiforms{} are fixed length, because they contain
  clauses from argument \psiforms{}, and each subset \psiform{} of a
  fixed length \psiform{} is obviously a fixed length \psiform{}.
  \end{proof}
}

%{\noindent{\bf  Lemma \ref{lm:fixednooverlap}}
\begin{ourlemma}
\label{lm:fixednooverlap}
  Let \m{\psi_1} and \m{\psi_2} be fixed length \psiforms{}. In two
  different subset-matches of \m{\main(\psi_1)} onto
  \m{\main(\psi_2)}, no two different literals of \m{\main(\psi_1)}
  match the same literal of \m{\main(\psi_2)}.
\end{ourlemma}
\begin{proof} % of Lemma \ref{lm:fixednooverlap}

  As always, we assume that there is no overlap between the variables
  in two different \psiforms{}.  Suppose that the above statement is
  not true, i.e. there exist two different subset-matches of
  \m{\main(\psi_1)} onto \m{\main(\psi_2)} that match two different
  literals \m{d_1} and \m{d_2} of \m{\main(\psi_1)} on the same
  literal \m{d} of \m{\main(\psi_2)}.  Let \m{\sigma_1} and
  \m{\sigma_2} be substitutions corresponding to each subset-match,
  i.e.  \m{\sigma_1} and \m{\sigma_2} are in
  \m{\mgusubset(\main(\psi_1), \main(\psi_2), \vars(\psi_1))}.
  
  Consider the following substitution \m{\sigma}.
\begin{itemize}
\item If \m{d_1} and \m{d_2} do not share variables, construct 
\m{\sigma} as follows: combine bindings on variables in \m{d_1} from
\m{\sigma_1} and  bindings on variables in \m{d_2} from \m{\sigma_2}.
Then, obviously, \m{d_1\sigma = d_2\sigma = d}.
  
\item Otherwise, if \m{d_1} and \m{d_2} do share variables, rename
variables in \m{d_2} so that there is no overlap with variables in
 \m{d_1}.  Modify \m{\sigma_2} by renaming the variables in the same
 way we did with  \m{d_2}, and construct \m{\sigma} as in the previous
 case. Again, \m{d_1\sigma = d_2\sigma}.
\end{itemize}

Thus, both cases produced a contradiction to the fact that no two
literals of a fixed length \m{\psi_1} unify. 
\end{proof}
}
\noindent {\bf Observation \ref{lm:fixednummatches}}
\lemmaEight

\begin{proof}% of Observation \ref{lm:fixednummatches}

\noindent Suppose there are \m{i_k} literals in  \m{\main(\psi_2)} that matched the k-th literal of \m{\main(\psi_1)}.  Since according to Lemma 
\ref{lm:fixednooverlap} (page \pageref{lm:fixednooverlap})  no two different 
matches can match two different literals of \m{\main(\psi_1)} to the
same literal of \m{\main(\psi_2)},
\m{i_1+\ldots+i_k \leq C}, otherwise two literals of  \m{\main(\psi_1)} would 
match  the same literal of  \m{\main(\psi_2)}.

The maximum size of \m{{\mgusubset(\main(\psi_1), \main(\psi_2), \vars(\psi_1))}} is bound by the product \m{i_1\times\ldots\times i_k }. 
By the Cauchy's inequality \md{ \frac{i_1+\ldots+i_k}{k}\geq
(i_1\times\ldots\times i_k)^{1/k}.} 
  The product \m{(i_1\times\ldots\times i_k)} is limited by   
\m{(\frac{C}{k})^k} with the equality reachable only when
\m{i_1=i_2=\ldots=i_k = \frac{C}{k}}. Then the product \m{i_1\times\ldots\times i_k }.   The  maximum of this product is reached when  \m{\log(\frac{C}{k}) -1 = 0}, i.e. when  \m{\frac{C}{k} = e}, and equals \m{e^{C/e}}.
  
Thus, when the maximum number of disjuncts in a \psiform{} is \m{C}, number of possible subset-matches is bounded by \m{e^{C/e}}.  
%To find the order of the maximum value of the product we assume that
%\m{i_1,\ldots ,i_k \leq C} are real numbers each equal to \m{\frac{C}{k}}.
\ignore{ %shortened
Then the product \m{i_1\times\ldots\times i_k } equals 
\m{(\frac{C}{k})^k}. To find the maximum of this function, calculate the
derivative of \m{\log(\frac{C}{k})^k = k \log(\frac{C}{k})} with respect to
\m{k}: 

\md{ (k \log\frac{C}{k})' = - k\times\frac{k}{C}\times \frac{C}{k^2} +
\log(\frac{C}{k}) = 
	\log(\frac{C}{k}) -1.
}

The second derivative  \m{(-\frac{C}{k^2}\times \frac{k}{C})} is negative, so
the graph of the function is concave and  therefore the  maximum of the
function is reached when  \m{\log(\frac{C}{k}) -1 = 0}, i.e. when
\m{\frac{C}{k} = e}, and equals \m{e^{C/e}}.
  
Thus, when the maximum number of disjuncts in a \psiform{} is \m{C}, number of possible subset-matches is bounded by \m{e^{C/e}}.  
}
%\theend
\end{proof}
}

\noindent {\bf Lemma \ref{lm:saturate}}\lemmaSeven

\begin{proof} %of Lemma \ref{lm:saturate}
  
  The SOK returned by {\bf Saturate} (Figure \ref{fig:saturate}) contains the input set of
  propositions \m{s} and some additional propositions that are
  derived from \m{ s} using unit clause resolution, i.e. those
  that follow from \m{s}. Thus the returned SOK \m{s_0} is
  equivalent to the input.
  
  It is saturated because we compute and add the results of all
  possible resolutions to \m{s_0}. Thus, for every ground proposition \m{p}
  such that \m{s\entails p}, there is a  proposition
  \m{c\in s_0} such that \m{c\entails p}.
  
  {\bf Saturate} computes all possible resolutions in \m{s} and
  returns {\bf fail} whenever an empty disjunct is derived, as follows
  from the the known property of resolution deduction (see
  \cite{genesereth-nilsson} page 87): If a set \m{\Delta} of ground
  clauses is unsatisfiable, then there is a resolution deduction of
  the empty clause from \m{\Delta}.

To estimate the time complexity bound, we consider the following stages of the algorithm.
During the first stage, for each of n \psiforms{} in \m{s} the procedure will first compute the resolution with every atom in \m{s}, when the resolution rule is applicable. Determining if resolution between an atom and a single fixed length \psiform{} is applicable consists of computing an image of a single literal onto a \psiform{} (step 4 in Figure \ref{fig:saturate}), which takes constant time, assuming the number of exceptions, clauses and variables in a \psiform{} are constant bounded. 
Thus, the first stage takes time \m{O(mn)}.

Note that the result of each resolution is another \psiform{} (denoted \m{\psi_{new}} in the algorithm), which is added to the saturation \m{s_0}. 
For each \psiform{} at most \m{m} new \psiforms{} can be added to \m{s_0} as a result of resolution with the atoms in \m{s}. Furthermore, each of the added \psiforms{} will have 1 fewer literals in the main clause than the original. Overall,  \m{nm} new \psiforms{} with the maximum clause length \m{C-1} could be added to \m{s_0} during the first stage.

During the second stage, resolutions are computed between the \psiforms{} added in the previous stage and \m{m} atoms of \m{s}. This process will take time 
\m{O(m^2n)} and  add no more than \m{m^2n} new \psiforms{}  with the maximum clause length of \m{C-2}.

The third stage will take \m{O(m^3n)} time and add no more than \m{m^3n} new \psiforms{} with the clause length \m{C-3}, and so on.
\corr{2}{
Since the maximum possible length of the main clause in the \psiforms{} added at each stage is decreasing by one at each stage of this process, it is evident that the number of stages is bounded  by the size of the longest \psiform{} clause \m{C}. Overall computation will thus take time \m{\bigo(mn+m^2n+\ldots+m^Cn) = \bigo(m^Cn)}.
 }    
\end{proof}

%%%%%%%%%%%% psiplan!

\noindent{\bf  Theorem \ref{th:update}}
\restate{\thrmEleven}

{\begin{proof} %of Theorem  \ref{th:update}

We start by proving that the result of updating a saturated SOK is a
saturated SOK.   
We first show that if \m{s} is saturated  then \m{s_1= ((s \diff
{\assertlist^-}(a)) \diff \assertlist(a))} is also saturated (
recall that \m{\mathbf{{\assertlist}^-(a)}} is used to denote the set of negations of propositions in the assert list of \m{a}).
Suppose this is not true, i.e. there's a ground \psiplan{} proposition \m{p} such that, while
\m{s_1\entails p },  \m{\ourforall{p'\in s_1}p' \not\entails{}p
}. Let \m{q} be a smallest (non-empty) subclause of \m{p} such that \m{s_1\entails
q} (there might be several such \m{q}). Since \m{s_1\subseteq s},
 \m{q}  must also be entailed by \m{s}, but \m{s} is saturated, so
 there exists a \m{q'} in \m{s} such that  \m{q'\entails q}, i.e.  
\m{q'\subseteq q}.

 \m{q'\not\in s_1} (otherwise \m{q'} as a subclause of \m{p} would
entail \m{p}) so \m{q'} must be entailed by either  \m{\assertlist(a)}
or  \m{\assertlist^-(a)}.  We abbreviate the union
\m{\assertlist(a)\cup{}{\assertlist^-(a)}} by
\m{\closure\assertlist(a)}.    
%Otherwise, if some of literals do not appear in any kn-propositions of \m{s},
%it is possible to find a k-state model of \m{s_1} in which 
%\m{\kn(q)} is \m{\false}.
%Since \m{\kn(q')\entails \kn(q)}, \m{q'} is a subclause of \m{q}. 
Since \m{q'\in ({\image {\assertlist(a)}{s}}) \cup( {\image{
\assertlist^-(a)} {s}})}, there must be a literal \m{e} in
\m{\closure\assertlist(a)} such that \m{e} is a subclause of  \m{q'}, and
therefore, \m{e} is a subclause of  \m{q}.
Note, that %for every kn-proposition {\kn(t)} entailed by \m{s_1}
 since \m{s_1\entails q}, in case \m{q\not\in s_1} there must be a way of
deriving \m{q} by resolution from some propositions of \m{s_1}, which is only possible when there exists a proposition \m{r} in \m{s_1} such that \m{r}
 contains \m{q} as a subclause. \ignore{(To see this note that if \m{q\in{}s_1} then \m{r=q}. Otherwise, since for any subclause \m{q'} of \m{q}, \m{s_1\not\entails{}q'}, {q} is derived from \m{s} by resolution. Thus, there is a clause \m{r\in{}s} such that \m{q\subseteq{}r}.)} This means that \m{r} has \m{e} as a
subclause, and consequently \m{r} is entailed by \m{e}. But
according to  the definition of \m{s_1}, it does not contain any
clauses entailed 
by any clause in \m{\closure\assertlist(a)}. We arrive at a
contradiction, so \m{s_1} is saturated. 
  
Adding \m{\assertlist(a)}, which consists of literals and  is itself saturated, to \m{s_1} also produces a saturated state.
 Assume there is a proposition \m{q}
that is not entailed by either \m{s_1} or some element of
\m{\assertlist(a)}, but is entailed by
\m{s_1\cup{\assertlist(a)}}. \m{q} cannot be an atom, therefore it is
 a negated clause. The only clauses that are not entailed by
 \m{\assertlist(a)} and  \m{s_1} separately, but are entailed by their
 union are those obtained via resolution of some atom \m{e\in\assertlist(a)}
with a ground clause of the form \m{\neg{}e\vee x} in  \m{s_1}. But
 this is impossible, because \m{ \assertlist^-(a)\entails\neg{}e\vee
 x}, so such  clause would not be in \m{s_1}. We arrive at a contradiction. 

In case \m{s} was minimal, \m{s'} is also minimal, because
\begin{itemize}
\item removing clauses from a minimal set preserves minimality, so \m{s_1}
is minimal, and 
\item \m{s' = s_1\cup{\assertlist(a)} } is minimal because
\begin{enumerate}
\item \m{s_1} does 
not contain any propositions entailed by any literal in \m{\closure\assertlist(a)}, 
\item \m{\assertlist(a)} is minimal, and 
\item \m{s_1} does not entail anything in
\m{\assertlist(a)}.
\end{enumerate}
\end{itemize}

To prove that the \m{update} function is correct and complete, we need
to show that  for \m{s'= update(s,a)}: 
\begin{equation}
\Ms(s') = do (a, \Ms(s)).
\end{equation}

\ignore{\em For the purpose of this proof, instead of representing a
world with a set of atoms and making the closed world assumption, 
we will assume  that each world \m{w} is represented by a complete set of
literals that are true in the world. These two representations are
equivalent.}

{\em Completeness proof.} We first show that \m{ do (a,
\Ms(s)) \subseteq \Ms(s') }, i.e. for every world \m{w} in
\m{\Ms(s)}, its successor,  \m{w' = do (a,w)}, is  in \m{\Ms(s')}.    
The set of possible worlds consists of all and only worlds that
model the agent's knowledge of the world, i.e. for any \m{s} \m{\Ms(s) = \set{w\ourst
(p \in s) \implies w(p) = true}.}
Thus, to show that \m{w'\in\Ms(s')} we need to prove, that for every
proposition \m{p} in \m{s'},  \m{w'(p)=\true}.

Note that according to the world transition model, \m{w'= (w -
\closure{\assertlist}(a)) \cup {\assertlist(a)}}.

We partition \m{s'} into \m{s'_1 =((s \diff{\assertlist^-}(a)) \diff
 \assertlist(a)) } and \m{s'_2 = \assertlist(a)}. We partition
\m{w'} into \m{w'_1 = w - {\assertlist^-}(a)- {\assertlist}(a)} and
\m{w'_2= {\assertlist}(a)}.
Since \m{w\in\Ms(s)}, for every \m{p_1} such that \m{p_1\in s'_1},
 \m{w'_1(p_1)}. Also, for each \m{ p_2 \in s'_2}, we have
 \m{w'_2(p_2)}. Therefore for every \m{p} such that \m{p\in s},
\m{w(p)}. 
 
{\em Correctness proof.}  Now we need to show that 
 \m{\Ms(s')\subseteq do(a, \Ms(s))}, i.e. every possible world  \m{w'}
of \m{s'} has a predecessor \m{w} that is a possible world of \m{s}.
We need to show that for every \m{w' \in \Ms(s')} there is a world 
\m{w} such that \m{w' = (w - \closure{\assertlist}(a)) \cup
\assertlist(a) } where \m{w} is in \m{\Ms(s)} and 
\m{\closure\assertlist(a)} denotes the union \m{\assertlist(a)\cup{}{\assertlist^-(a)}}. A possible world
is a model of all propositions  \m{p} such that \m{p\in s},
i.e. \m{w} is in \m{\Ms(s)} if and only if \m{w} models every such
domain proposition \m{p}.

The proof is by construction. Since \m{s} is saturated,  for every
proposition \m{p} that is implied by \m{s}, there's a single
proposition \m{q\in s} such that \m{q\entails p}.

STEP 1. Since \m{w' = do (a,w)}
we need to include in \m{w} all literals of \m{w'} that are not in
\m{{\assertlist (a)}}, because those would not have changed as a
result of the action. Let \m{w_0 = w' - {\assertlist}(a)} and \m{w} will include \m{w_0}.

STEP 2. We also include in  \m{w} those literals from
\m{\closure{\assertlist (a)}} that are {\em known} in \m{s},
i.e. the literals \m{l\in \closure{\assertlist} (a)} such that \m{l
\in s}.  

STEP 3. At this point every literal or its complement is included in
\m{w} 
except for \m{l\in \closure{\assertlist}(a)} where neither \m{l} 
nor \m{\neg l} belongs to \m{s}. We now describe  a procedure for choosing 
either the literal or its complement for inclusion in \m{w} from these
``leftover'' literals. Suppose  \m{\neg l} is an arbitrary negated
literal from this set. Further, let \m{C = {\image {\neg l}
s}}. If there is 
a proposition in \m{C} that is not already implied by some \m{p},
where \m{p\in w}, then we must
include \m{\neg l} in \m{w} in order to keep it accessible from \m{s}.
Otherwise we may include in \m{w} either \m{l} or \m{\neg l}.  

The world \m{w} is now completely specified and is easy to verify that 
\m{w\in\Ms(s)}, as well as \m{w' = do(a,w)}.
\ignore{%to shorten
\begin{enumerate}
\item \m{w\in\Ms(s)},  since
\begin{itemize}
\item 
For all \m{p\in (s\diff \assertlist^- (a))\diff
\assertlist (a)}, we have  \m{w(p)=\true}, because 
\md{(s\diff \assertlist^- (a))\diff \assertlist (a) = (s'\diff
\assertlist^- (a))\diff \assertlist (a),} 
for all \m{p\in (s'\diff \assertlist^- (a))\diff \assertlist (a)}
 \m{w'(p) =\true},  
and \m{w} includes \m{w' - \assertlist(a)}.
\item At STEP 2 we added to \m{w} those literals that are known in
\m{s}, and therefore are true in all of its possible worlds,
\item For each  literal \m{\neg l} (or \m{l}) added at STEP 3, neither \m{l } nor \m{\neg l} are in \m{s} (otherwise it would have been added to \m{w} at
STEP 2). However, the literals added to \m{w} at STEP 3. ensure that 
each proposition \m{\neg{}a_1\vee\ldots\vee\neg{}a_k}  in \m{s}, such that 
the value of \m{\neg{}a_1\vee\ldots\vee\neg{}a_k} is not yet
completely defined by \m{w} (because  STEP 2 leaves  \m{w} incomplete),
is true in \m{w}.  
\end{itemize}
and therefore, \m{w} is a possible world for the SOK \m{s}.     
\item \m{w' = do(a,w)}, because 
\m{w'} and \m{w} only differ in values of
literals in \m{\closure\assertlist(a)} in a way that is consistent with \m{a}. 
\end{enumerate}
}
\end{proof} 
}

\ignore{
%%%PSIPOP proofs

{
\noindent {\bf Lemma \ref{lm:splits}}\lemmaNine

\begin{proof} of Lemma \ref{lm:splits}

  Both of these procedures replace a \psiform{} goal \m{\psi_g} with a
  set of goals \m{(\image{\psi}{\psi_g})} and \m{(\psi_g \diff \psi)}
  for some \psiform{} \m{\psi}. Since \m{\psi_g
    =(\image{\psi}{\psi_g})\cup (\psi_g \diff \psi)}, this
  transformation is equivalent.

\end{proof}
}

{
\noindent {\bf Lemma \ref{lm:psipopsound}}
\lemmaTen

\begin{proof} of Lemma  \ref{lm:psipopsound}

  Suppose \m{S_{i_1}, \ldots, S_{i_k}} is some ordering of steps in
  \m{P} that respects the partial ordering \m{O}.

Correctness and completeness of the update rule guarantee that 
any ordered sequence of actions \m{S_{i_1}, \ldots, S_{i_k}} 
  executable in the agent's model from a SOK \m{s_0} that is
  consistent with \m{\cal I},  is also executable in the actual
  world. Therefore, to show executability of the \m{S_{i_1}, \ldots,
    S_{i_k}} we only need to show that for every \m{i_j},
  \m{update(S_{i_1} \ldots S_{i_{j-1}}, s_0) \entails \precond
    (S_i{_j})}.

To show that  the plan achieves the goal it suffices to show that the final SOK
  \m{update(S_{i_1} \ldots S_{i_k}, s_0)}, entails \m{\cal G}. This
  would imply that \m{\cal G} is true in all possible worlds of the
  final SOK.

\ignore{ The proof is by induction on the number of iterations of
  \psipop, \m{m}.  We show that after \m{m} iterations
\begin{itemize}
\item the set of orderings \m{O} contains no contradictions, and
\item if \psipop{} returns a partially ordered plan \m{P}, any
  candidate plan \m{S_{i_1}, \ldots, S_{i_k}} is a solution plan.
\end{itemize}

Recall, that \psipop{} initially is called with a ``dummy'' plan,
where the START step has no preconditions and has assert list encoding
the initial SOK \m{s_0=\cal I}. The FINISH step has no assert list and
its effects encode the goal conditions \m{\cal G}.

The least number of iterations for which \psipop{} returns with a
successful plan for a non-empty goal is \m{m=2}. The algorithm can
return a plan after 2 iterations if there is a single precondition in
the FINISH step, which was entailed by some effect of the START step,
or some effect of a new step that has no preconditions. The
constructed plan would be correct and executable. If the algorithm did
not return, the set of orderings would contain the ordering of step
START before the FINISH, and possibly the ordering of another action
between these two steps, which is consistent.

Suppose that after \m{m} iterations the ordering of steps contains no
contradiction and if the algorithm returns a plan, it is executable
and achieves the goal.

Suppose the algorithm did not return with a plan at the \m{m}-th
iteration, and returned after \m{(m+1)}-st iteration. In such case it
either
\begin{itemize}
\item returned {\bf fail}, or
\item returned a plan.
\end{itemize}
}

We now show that if a plan is returned, then for any step \m{S_{i_c}
  }, including the FINISH step, for any ordering of steps that
respects \m{O}, if \m{s_c} is the SOK immediately preceding \m{S_{i_c}
  }, \m{s_c\entails\precond(S_{i_c})}.

Since all preconditions of all steps have at some point been added to
the open list, each precondition was at some point picked and removed
from it (at step \ref{PickActionStep}) and \psipop{} either found a
link to it from some effect of some step, or \psipop{} split it into
an equivalent set of propositions (see Lemma \ref{lm:splits}), all of
which have been linked from some steps in \m{S}.  Suppose without loss
of generality, that \m{c} is a whole or a part of some precondition \m{p}
on step \m{S_{i_c}}, for which there is a link \m{{\nmclink{i_e} e c
    {i_c}}\in L}.  Since each causal link imposes an ordering of the
source step before the target, \m{S_{i_e}} precedes \m{S_{i_c}} in
\m{O}. Thus, for any order \m{S_{i_1}, \ldots, S_{i_k}} of the steps
in the plan we have to show the following
\begin{enumerate}
\item the SOK \m{s_e=update(S_{i_1} \ldots S_{i_e}, s_0)} contains \m{e},
  and since \m{e\entails c}, therefore \m{s_e\entails c},
\item  for any ordered
  sequence \m{\vec a} of the steps \m{S_{i_e+1}, \ldots, S_{i_c-1}},
  that are the all and only steps of plan \m{P} that can occur between
  \m{S_{i_e}} and \m{S_{i_c}}, \m{update(\vec{a}, s_e)} entails \m{c}.
\end{enumerate}

The first of the above two statements follows from the fact that
effect \m{e} is added to the SOK according to the update rule. The
proof of the second statement follows.  Suppose there is some sequence
\m{\vec a}, for which \m{update (\vec{a}, s_e)} does not entail \m{e}.
This means that \m{e} (or part of \m{e}, in case \m{e} is a quantified
\psiform{}) has been removed from \m{s_e} as the result of an update
and no proposition that entails \m{e} (or that part of \m{e}) was
added. By definition of the \m{update} function (\ref{eq:update})
this is only possible if there is a step \m{S_{i_t}} in \m{\vec a}
with an effect \m{t\in \assertlist(S_{i_t})}, such that
\m{{\image{(\neg t)} {e}}\neq\emptyset}.  But in this case \m{t} would
be a threat to the link \m{\nmclink {i_e} e c {i_c}}, unless \m{\image
  {({\image{(\neg t)} {e}})} {c} =\emptyset}.  If \m{\image
  {({\image{(\neg t)} {e}})} {c} \neq \emptyset}, we arrive at a
contradiction with the fact that the returned plan does not contain
any threats, otherwise, if \m{\image
  {({\image{(\neg t)} {e}})} {c} =\emptyset}, \m{e\diff(\neg t)} entails \m{c}, and so does
\m{update(\vec{a},s_e)}.

Since \psipop{} returns {\bf fail} whenever an inconsistency in the
orderings occurs, every returned plan has a consistent set of
orderings \m{O}.

\end{proof}
}

%%% File completeness.tex

{\noindent {\bf Lemma \ref{ContractionLemma}}\lemmaEleven

\begin{proof}of Lemma \ref{ContractionLemma}

Let \m{s_0 = {\cal
I}} and \m{s_1} denote the SOK \m{update(S_1,s_0)}.
According to the definition, to show that  \m{\set{S_2, \ldots, S_n}}  is a
solution to the planning problem \m{\pp {\Lambda, s_1} {\cal G}}, we must show that this 
sequence of actions is executable from any world described by \m{s_1} and
that  the goal is true in any world resulting from executing the sequence in any of the worlds described by \m{s_1}. 

Since our update rule is correct and complete,  it suffices to show the following. 
\begin{enumerate}
\item The preconditions of each action \m{S_j}, where \m{2\leq j\leq n},
 are entailed by the SOK \m{update(S_2\ldots S_{j-1},s_1)}.
\item The goal is entailed by the SOK \m{update(S_2\ldots S_n,s_1)}.
\end{enumerate}

Since  \m{S_1, \ldots, S_n} is a solution to  the planning problem
\m{\alpha = {\pp {\Lambda, \cal I} {\cal G}}}, we have 

\begin{itemize}
\item  For all \m{S_j}, where \m{1\leq j\leq n}, \m{S_j} is executable in
every world resulting from executing \m{S_1,\ldots,S_{j-1}} in any world of
\m{\Ms(s_0)}, therefore 
\begin{equation}\label{eq:1}
update(S_1\ldots S_{j-1}, s_0) \entails \precond(S_j) \mbox{ for all
}j, \mbox {  such that  } 1\leq j\leq n.
\end{equation}
Since  our update rule is correct and complete, or in other words it neither ``loses'' nor adds possible worlds 
\begin{equation}\label{eq:2}
update(S_1 \ldots S_{j-1},s_0) = update(S_2\ldots  S_{j-1}, s_1) , 
\end{equation}
where  \m{s_1=update(S_1,s_0)}.
So from (\ref{eq:1}) and (\ref{eq:2}) we have
\md{update(S_2\ldots S_{j-1}, s_1) \entails \precond(S_j) \mbox{ for all
}j, \mbox {  such that  } 1\leq j\leq n.} Therefore each action in the plan
\m{S_2,\ldots,S_n} is executable. 

\item \m{update(S_1\ldots S_n, s_0) \entails {\cal G}}, and therefore 

\md{update(S_2\ldots S_n, s_1) \entails \cal G,} so the plan
\m{S_2\ldots S_n} also achieves the goal.
\end{itemize}
\end{proof}
}

\noindent{\bf  Theorem \ref{th:completeness}}
\thrmTwelve

{\begin{proof} of Theorem \ref{th:completeness}

 We use induction on the number of steps \m{n} in the solution
\m{S_1, \ldots, S_n}.

1. {\em Base case:} n = 0. This means that the goal \m{{\cal G}} follows from
the initial SOK \m{s_0} which is a saturated equivalent of \m{\cal I}, and no other steps except for the dummy START and FINISH steps are required. Since \m{s_0} is saturated, for every
proposition \m{p\in\precond}( FINISH), there is an effect \m{e} in
\m{\assertlist}(START) such that \m{e} either entails or nearly entails \m{p}.  
For every atom goal \m{a} there must be an effect \m{a} on the START step, and \psipop{} will create an appropriate link.

By Theorem \ref{th:Entailmentthrm} (page \pageref{th:Entailmentthrm}), since \m{\psi} is entailed  from the set of \psiforms{} in \m{s_0}, there  exists a \psiform{} \m{\psi_i \in s_0} that nearly entails   \m{\psi}. Goal Splitting separates the part of  \m{\psi} that is entailed by \m{\psi_i}, from the e-difference  \m{\psi\diff\psi_i}, posting \m{\psi\diff\psi_i} on the list of open goals, \m{open}. By the virtue  of the non-deterministic choice, \psipop{} tries all possible ways of proving \psiform{} goals by splitting the goal according to {\em all} nearly entailing propositions in \m{s_0}. 
Thus, goal splitting is necessary for the completeness of \psipop{}.

Thus \psipop{} will create a link for every  
subgoal in \m{{\cal G}} from START, and the solution plan will be returned.

2. {\em The inductive step.} Assume that the theorem is true for any
sequence of at most \m{n-1} steps, i.e. for any planning problem
\m{\alpha}, if there is a solution plan of size less or equal to \m{n-1},
\psipop{} will return a  compatible partial plan.
 We must now show that for any planning problem \m{\alpha = {\pp
{\Lambda}{\cal I,G}} } if a solution  \m{S_1, \ldots, S_n} of  
size \m{n} exists, \psipop{} will return a partial plan  that is compatible with \m{S_1, \ldots, S_n}. 

%Suppose \m{\set{S_i}_{i=0}^n} is the solution to be found.
Let \m{s_1} denote the SOK \m{update(S_1,s_0)} and  let \m{\alpha'} denote
the planning problem  \m{{\pp{\Lambda,s_1}{\cal G}}}.
By  Lemma \ref{ContractionLemma} above \m{S_2,\ldots,S_n} is
a solution to \m{\alpha'} and by the inductive assumption \psipop{} will
return a partial plan \m{P'} that has a candidate plan
\m{S_2,\ldots,S_n}.  
%\m{P} is very similar to \m{P'} and w
We will show how \psipop{} constructs a partial plan 
\m{P} where \m{P} is very similar to \m{P'}  by examining the choices it made when constructing \m{P'}% with some differences
 ( figures \ref{fig:cp-fig1}-\ref{fig:compl-3} illustrate this
construction). The differences concern the links of \m{P'} that originate 
from its initial step which we call START', whose assert list is \m{s_1}.

We  break up this set of links into  two subsets:
\begin{itemize}
\item \m{L_l} -- links supporting a literal, and
\item \m{L_q} -- links supporting a quantified \psiform{}.
\end{itemize}

We further partition the links \m{{\clink {START'} e c {S_j}}} in \m{L_l} as
follows 
\begin{itemize}
\item \m{L_l^0 = \set{{\clink {START'} e c {S_j} }\ourst s_0\entails c}},
\item \m{L_l^1 = \set{{\clink {START'} e c {S_j} }\ourst s_0\not\entails c}}. 
\end{itemize}

When \psipop(\m{\alpha}){} needs to find support for a subgoal that in
\m{P'} was supported by a link from \m{L_l} to a literal, we direct the algorithm instead to draw
the link from the step \m{START} in case  the original link was from
\m{L_l^0}, and from \m{S_1}, if it was  from  \m{L_l^1}. All threats to these
links can be resolved in the same way they were resolved in \m{P'}.

Now consider the links supporting quantified propositions,
i.e. \m{L_q}. Since the assert list of any action consists of literals only, when going from \m{P'} to \m{P},
all quantified \psiforms{} of \m{START'} ``move'' to  \m{START} with some
modification.  More precisely, according to the state update rule, for every
\m{\psi'\in s_1} there is a \m{\psi\in s_0} such that \m{\psi'} is 
\m{\psi} possibly with some exceptions added. Those exceptions are added
because of the effects of the step \m{S_1} and are exactly the set 
\ourmd{
\psi \diff \psi'= \set{\Psi\ourst \exists R \in \assertlist(S_1), \Psi = (\image {\neg 
R}{\psi})}}
See fig. (\ref{fig:cp-fig1}) for an example.

\begin{figure}[h!]
\input{cp-fig1.latex}
\caption{\m{\cal I} is the initial SOK, \m{S_1} is the first plan step, \m{s_1}
is the agent's SOK after performing \m{S_1} in \m{\cal I}, i.e. \m{Update(S_1, s_0)}.}
\label{fig:cp-fig1}
\end{figure}

Whenever \psipop(\m{\alpha}){}  needs to find support for a quantified
proposition \m{\psi_c} from a step \m{S_j, j>1}  that in \m{P'} was
supported by a link from 
\m{L_q}, \psipop{} will  find an appropriate \psiform{} in \m{s_0}, that nearly entails  \m{\psi_c}. Such a \psiform{} will always exist due to our 
observation above. Since \psipop(\m{\alpha'}){} found the supporting links to {\em 
all} ground propositions of \m{\psi_c},   \psipop(\m{\alpha}){} can draw 
supporting links in the same way, even though the splitting of \m{\psi_c}
could be different, because of the difference in the nearly supporting
propositions \m{\psi'} and \m{\psi}. Such a strategy will lead to the same
threats which can be resolved in \m{P} as they were in \m{P'}. The only {\em
new} threats are those that could come from effect \m{R}  on \m{S_1} to a link  \m{{\clink {START} {\psi}
{\psi_d} {S_j}}} from \m{\psi} in \m{s_0} to all or part of \m{\psi_c},
denoted here  
by \m{\psi_d}. Link splitting will eliminate the threat by 
separating out \m{(\image {\neg R}{\psi})} from the source and \m{\Psi =
\image {({\image {\neg R}{\psi}})} {\psi_d}} from the target and posting
\m{\Psi} to the list of open subgoals for step \m{S_j}.  The support to
the propositions in 
\m{\Psi} will be found as in \m{P'} in the effects of steps other than
\m{S_1}. Importantly, link splitting is the only threat resolution technique
we can use at this point. % apply in order to be able to generate the solution
%\m{\set{S_1,\ldots,S_n}} which we are seeking.
Promotion is not applicable, because \m{S_1} cannot
be ordered before \m{START}, and demotion would result in \m{S_j\prec S_1},
which would make the sought solution incompatible 
with the partially ordered plan \m{P}.  Link splitting results in ordering
\m{S_1} before \m{S_j}, which is consistent with the solution.  Thus link splitting is necessary for the completeness of \psipop{}.  Figures (\ref{fig:compl-1})-(\ref{fig:compl-3}) illustrate these ideas.
 
In addition, the preconditions of  \m{S_1} must be satisfied from \m{START}.
Since \m{S_1} is executable in \m{s_0}, satisfying \m{S_1}'s
preconditions from \m{s_0} is a planning problem with solution of size 0,
which is covered by the base case.

Any step that poses a threat to the new links from \m{START} to \m{S_1}
can be ordered after \m{S_1}, which is consistent with the ordering
in the solution to sequence of actions  \m{S_1, \ldots, S_n} that we
are trying to produce.

Thus, we have shown how \psipop{} will construct the solution to \m{\alpha}
that is compatible with \m{S_1,\ldots,S_n}. 
\end{proof}

\begin{figure}[h!]
\boxpage{\columnwidth}{
\input{cp-fig2.latex}}
\caption{Instances of \psiplan(\m{\alpha'}){}(top of the picture) and
\psiplan(\m{\alpha}){} working on partial plans \m{P'} and \m{P}, respectively. 
\m{\psi_c} is the next subgoal in both cases.}
\label{fig:compl-1}
\end{figure}

\begin{figure}[h!]
\boxpage{\columnwidth}{\input{cp-fig3.latex}}
\caption{Because of the differences in the nearly entailing \psiform{}, the
original goal is split differently in  \m{P'} and \m{P}.
\m{P} might contain threats that did not exists in \m{P'}. These new threats
are caused by \m{S_1}'s effects to the links from quantified \psiform{}
propositions in the effects of \m{START}.}
\label{fig:compl-2}
\end{figure}

\begin{figure}[h!]
\boxpage{\columnwidth}{\input{cp-fig5.latex}}
\caption{Finally,  propositions that were split from the
original \psiform{} goal in \m{P} are linked from the same steps as in
\m{P'}.}
\label{fig:compl-3}
\end{figure}

}

{
\begin{ourlemma}\label{lm:fixednooverlap}
  Let \m{\psi_1} and \m{\psi_2} be fixed length \psiforms{}. In two
  different subset-matches of \m{\main(\psi_1)} onto
  \m{\main(\psi_2)}, no two different literals of \m{\main(\psi_1)}
  match the same literal of \m{\main(\psi_2)}.
\end{ourlemma}
\begin{proof}  of Lemma \ref{lm:fixednooverlap}

  As always, we assume that there is no overlap between the variables
  in two different \psiforms{}.  Suppose that the above statement is
  not true, i.e. there exist two different subset-matches of
  \m{\main(\psi_1)} onto \m{\main(\psi_2)} that match two different
  literals \m{d_1} and \m{d_2} of \m{\main(\psi_1)} on the same
  literal \m{d} of \m{\main(\psi_2)}.  Let \m{\sigma_1} and
  \m{\sigma_2} be substitutions corresponding to each subset-match,
  i.e.  \m{\sigma_1} and \m{\sigma_2} are in
  \m{\mgusubset(\main(\psi_1), \main(\psi_2), \vars(\psi_1))}.
  
  Consider the following substitution \m{\sigma}.
\begin{itemize}
\item If \m{d_1} and \m{d_2} do not share variables, construct 
\m{\sigma} as follows: combine bindings on variables in \m{d_1} from
\m{\sigma_1} and  bindings on variables in \m{d_2} from \m{\sigma_2}.
Then, obviously, \m{d_1\sigma = d_2\sigma = d}.
  
\item Otherwise, if \m{d_1} and \m{d_2} do share variables, rename
variables in \m{d_2} so that there is no overlap with variables in
 \m{d_1}.  Modify \m{\sigma_2} by renaming the variables in the same
 way we did with  \m{d_2}, and construct \m{\sigma} as in the previous
 case. Again, \m{d_1\sigma = d_2\sigma}.
\end{itemize}

Thus, both cases produced a contradiction to the fact that no two
literals of a fixed length \m{\psi_1} unify.

\end{proof}
}

}

\ignore{
\noindent {\bf Procedure for generating random \psiforms{} for the experiments.}\label{proc:randPsi}

\noindent Here we present a brief description of the procedure used for generating random \psiforms{} for the entailment experiments described in Section \ref{sec:eval}.

The procedure returns a fixed length \psiform{} with  \m{c}
literals in the main clause, at most \m{v} variables, and \m{e}
exceptions, where \m{c,v} and \m{e} are the input parameters.
The \psiforms{} are created from
the predefined set of 14 predicate symbols 
with cardinality ranging from one to seven (two predicates per each
cardinality) and 20 constant symbols. Unless otherwise specified, all
random values involved are generated using a uniform distribution.

For each \psiform{} the procedure first generates the main clause of the
\psiform, and then the set of exceptions.

The main clause is generated by randomly selecting
the requested number of predicate symbols from the predifined set and
then generating the argument list for each predicate, based on the
number of variables \m{v}.
The argument list for each predicate is generated as follows. At
first, a list \m{\vars} of \m{v} fresh variables is created. For every 
predicate, each argument is either a randomly picked variable from \m{\vars} that has not yet been used as an argument for this predicate
\footnote{Recall that by definition of a \psiform{} a variable cannot
occur  in a \psiform{} literal more than once.}, or a constant
from the set of 20 predefined constants. While there are still some
variables  of \m{v} that have not been used in the predicate's
argument list, the chances of a variable versus a constant being
selected are fifty-fifty. When all variables of  \m{v} have been used,
the argument is always a constant. Note that this method of
generating a main clause may occasionally produce a clause 
with fewer variables than there are in \m{\vars}. In practice,
however, the number of variables in the resulting set of \psiforms{}
is roughly uniformly distributed. In case the resulting clause is not
a fixed length \psiform{} clause (as defined on page
\pageref{def:fixedLength}) the argument selection is repeated. 

To generate the exceptions, first, the number of variables instantiated
by the exception is selected at random between one and the actual
number of variables in the main clause. Then the algorithm randomly
selects a set of variables from the main clause and a list of
constants; selected variables and constants are 
paired together as a substitution to form an exception. 
}
